# Supplementary material for: DiffRF: Rendering-Guided 3D Radiance Field Diffusion
Source: arXiv:2212.01206 source file (2023-03-27)
Supplement: Supplementary file 1 [file 0_metadata_supp.tex]

\title{\vspace{-30pt}DiffRF: Rendering-Guided 3D Radiance Field Diffusion\\
- Supplementary Document -
}

\author{
Norman M{\"u}ller$^{1,2}$~~~
Yawar Siddiqui$^{1,2}$~~~ 
Lorenzo Porzi$^2$~~~
Lorenzo Porzi$^2$~~~
Samuel Rota Bul\`{o}$^2$~~~\\
Peter Kontschieder$^2$~~~
Matthias Nie{\ss}ner$^1$~~~
\vspace{0.2cm} \\
Technical University of Munich$^1$~~~
Meta Reality Labs Zurich$^2$
\vspace{0.2cm}
}
