# Supplementary material for: DiffRF: Rendering-Guided 3D Radiance Field Diffusion
Source: arXiv:2212.01206 source file (2023-03-27)

**DiffRF w/o 2D**

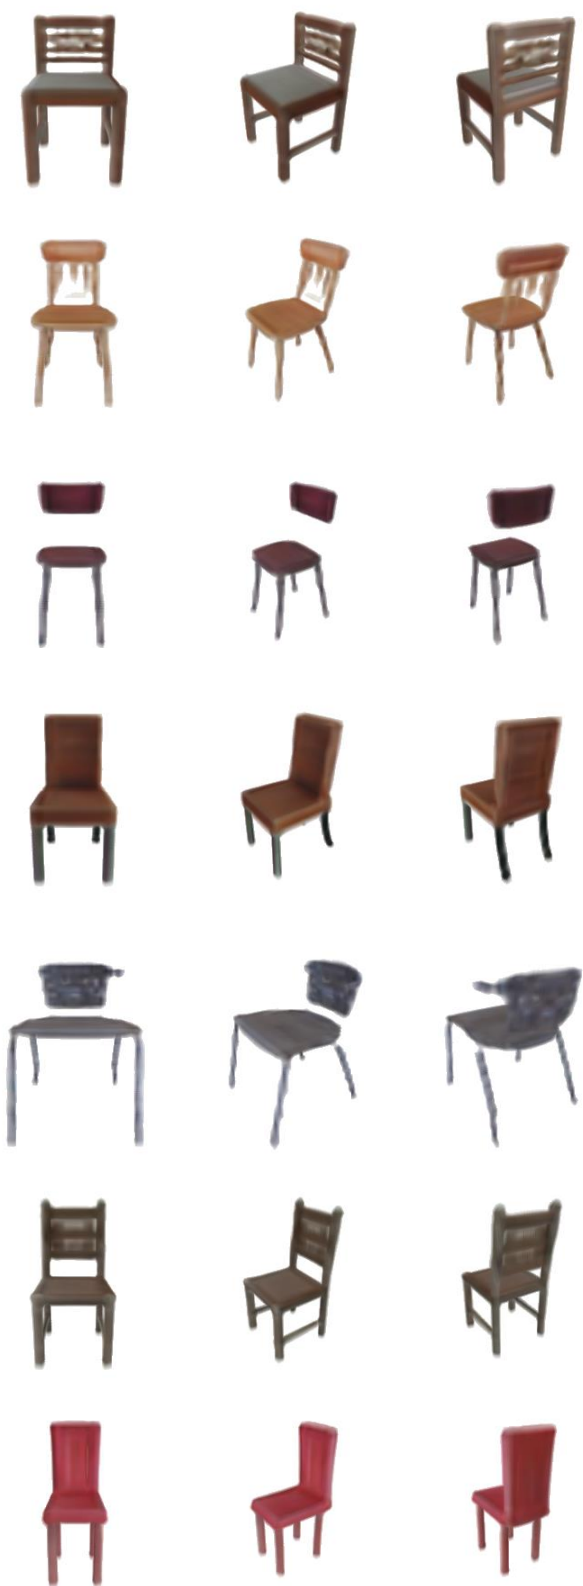

**DiffRF**

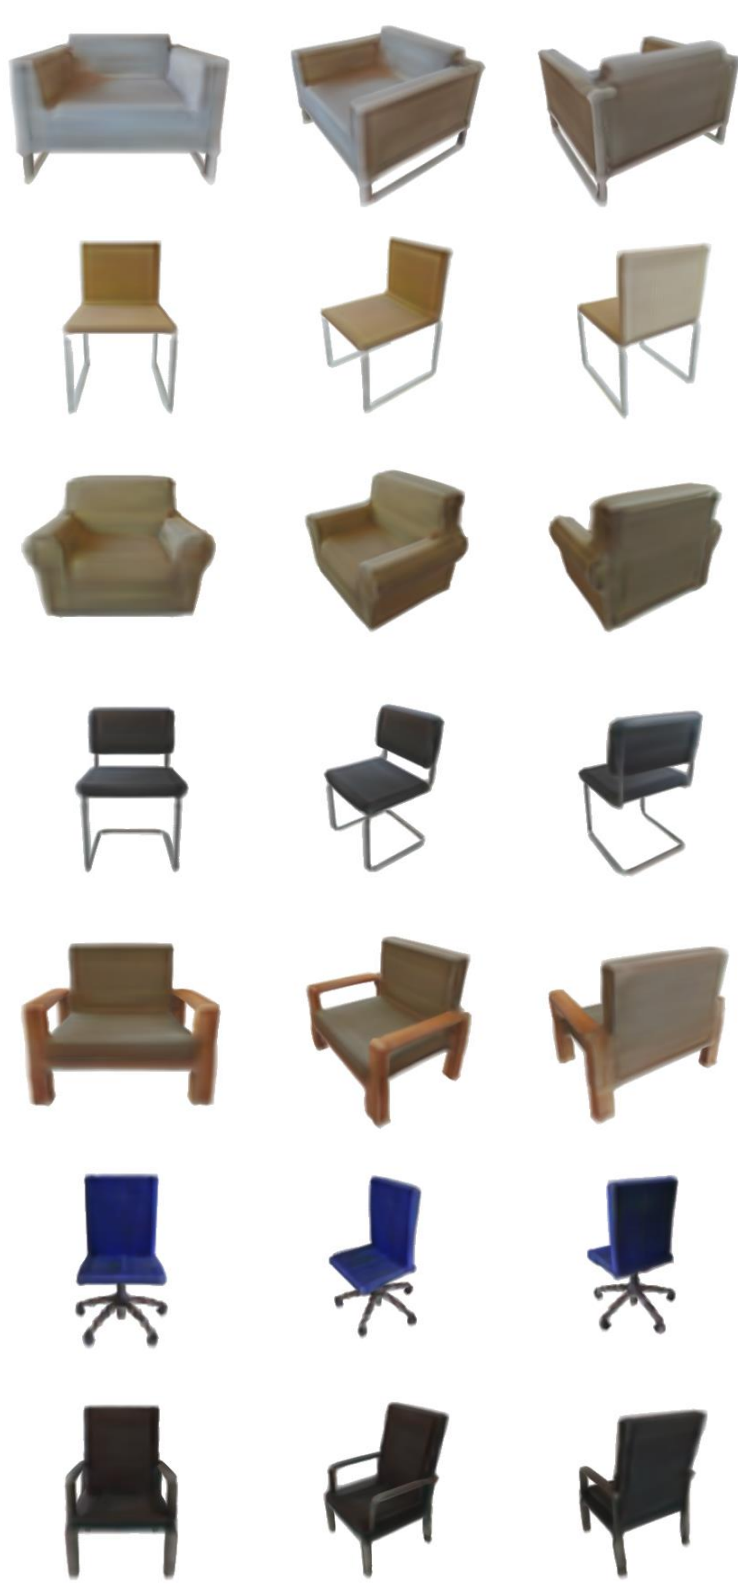

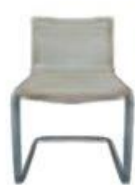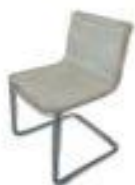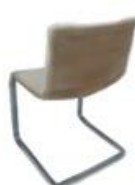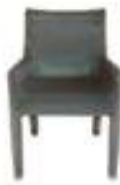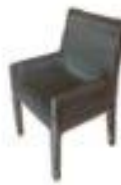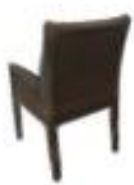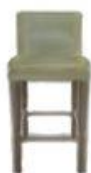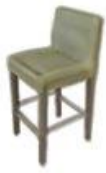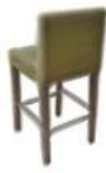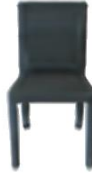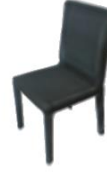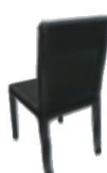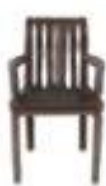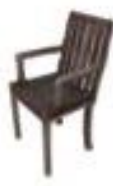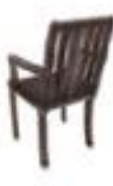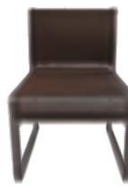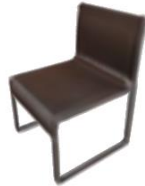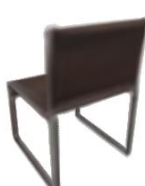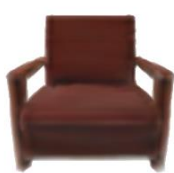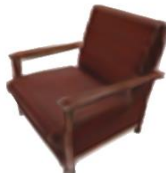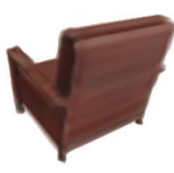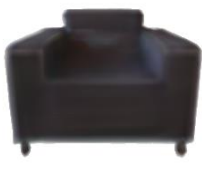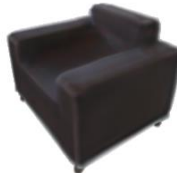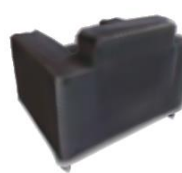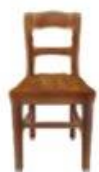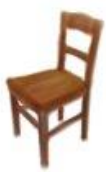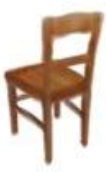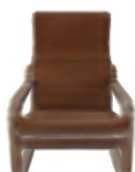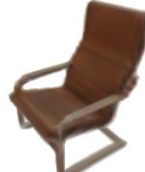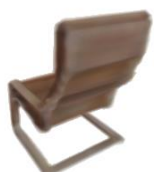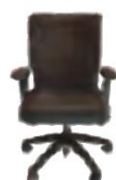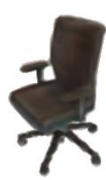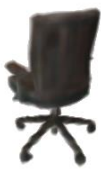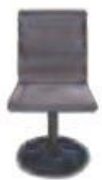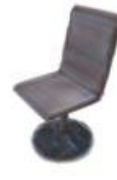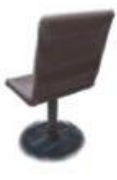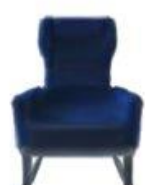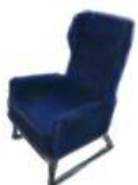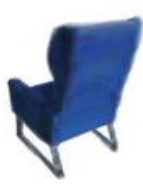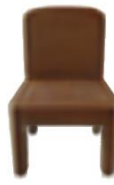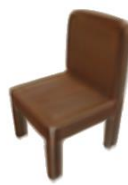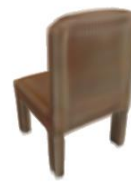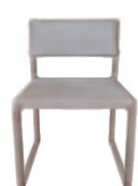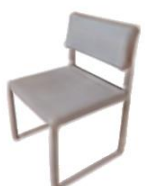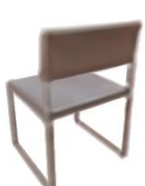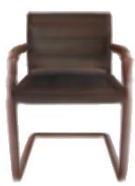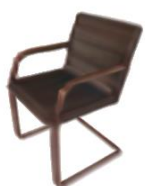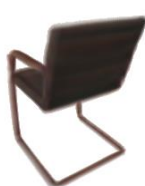

**DiffRF w/o 2D**

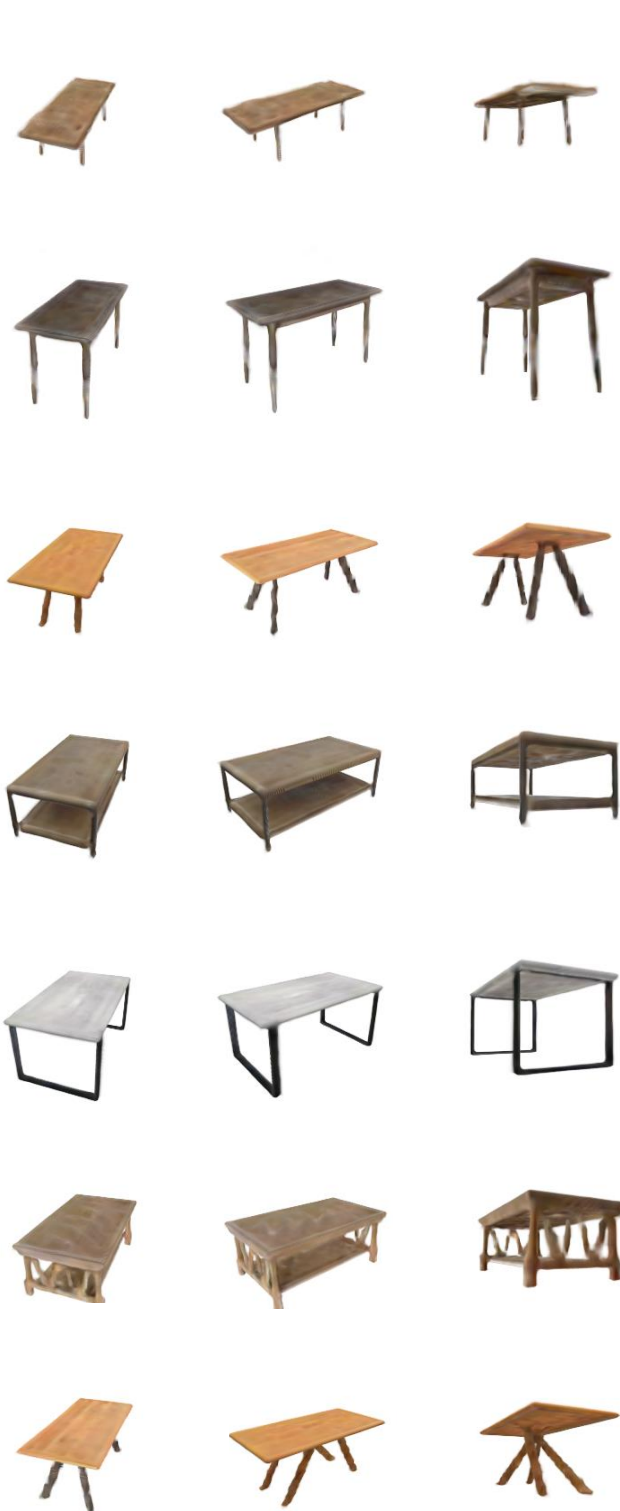

**DiffRF**

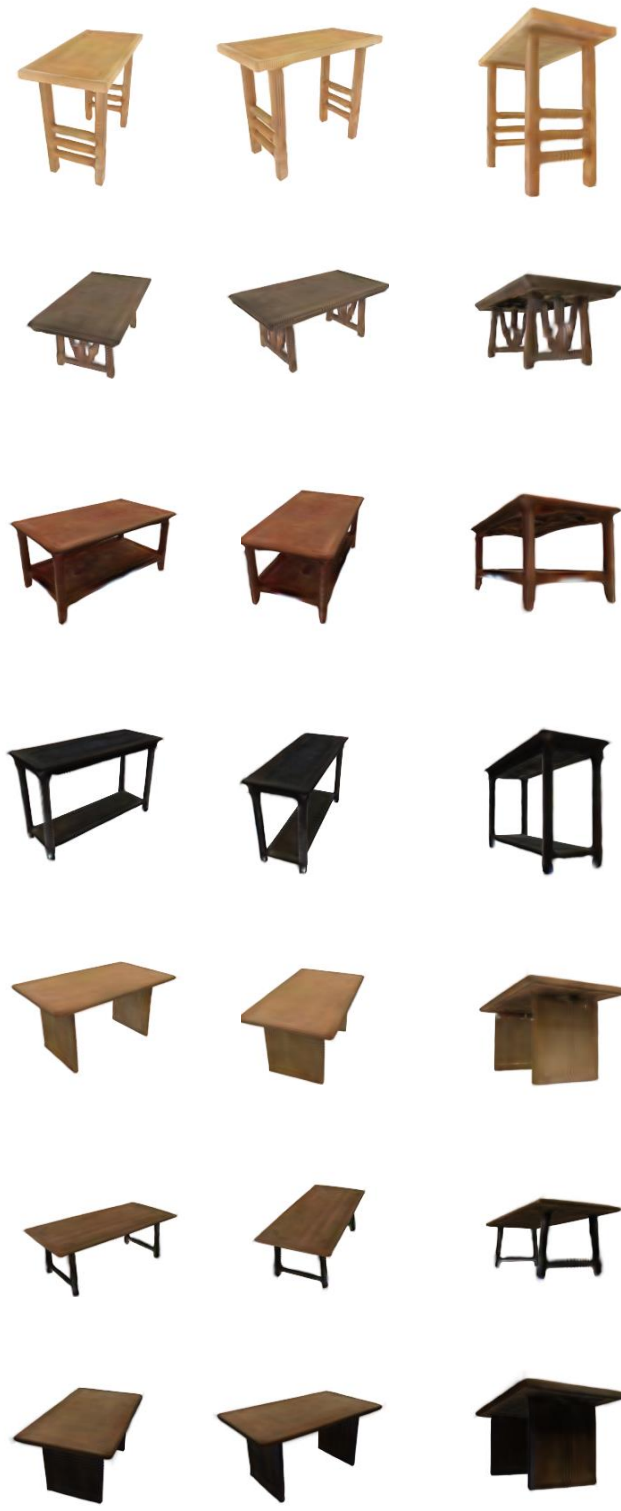

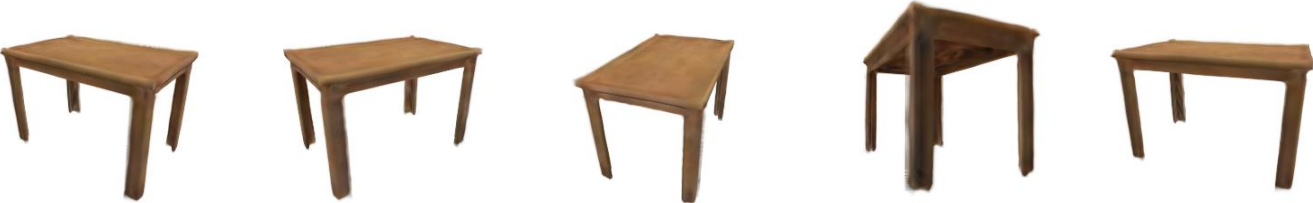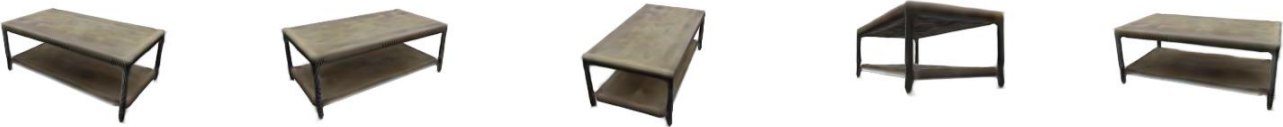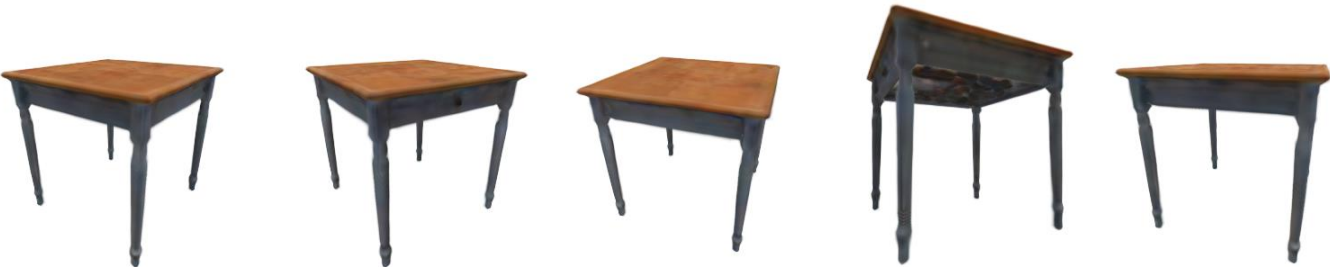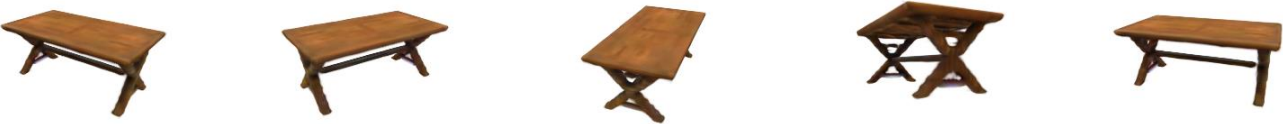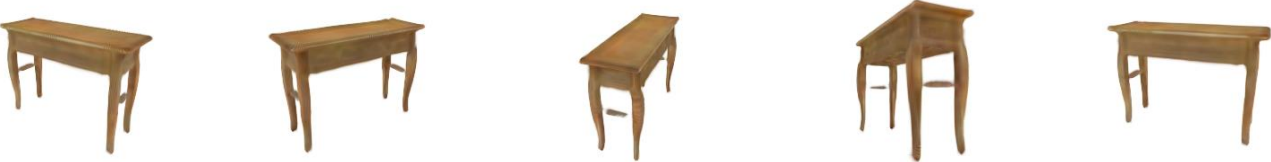

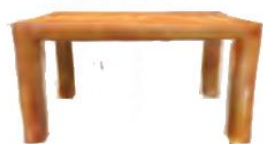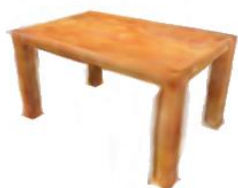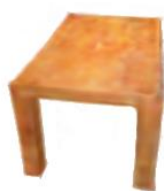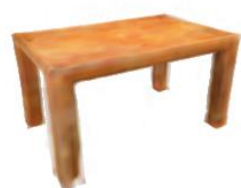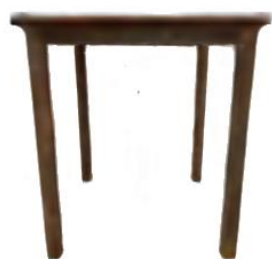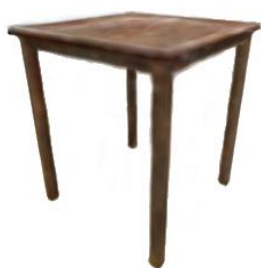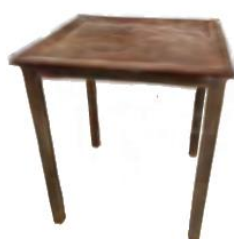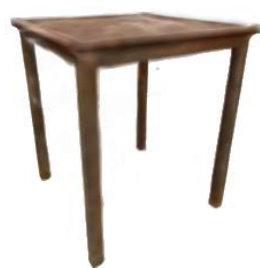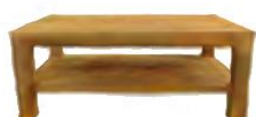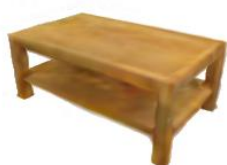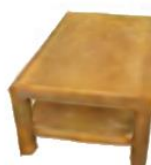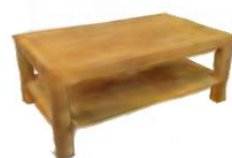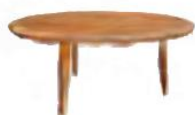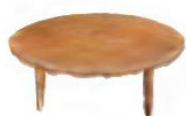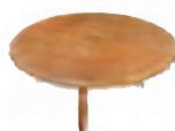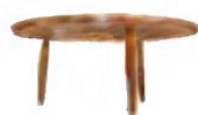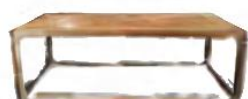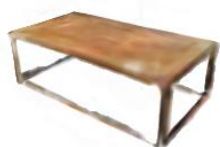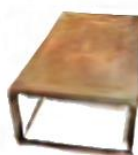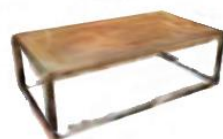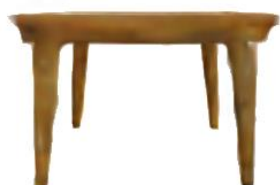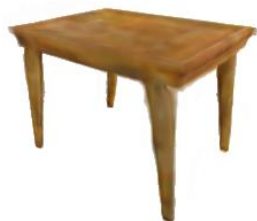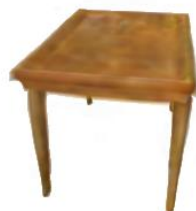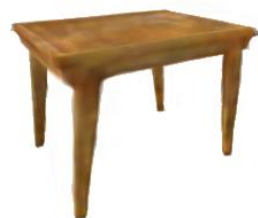



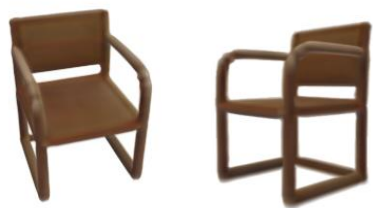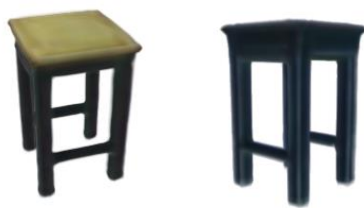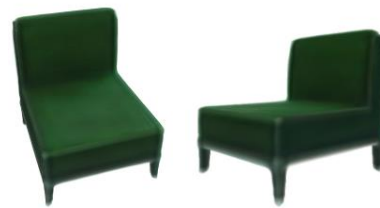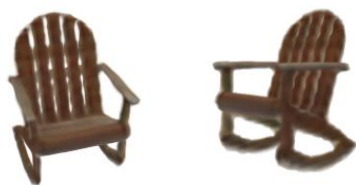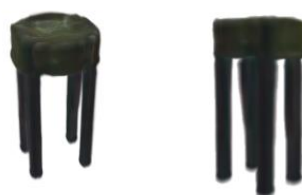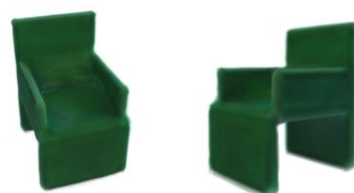

**a rustic simple wooden chair**

**a stool**

**a green comfortable chair**

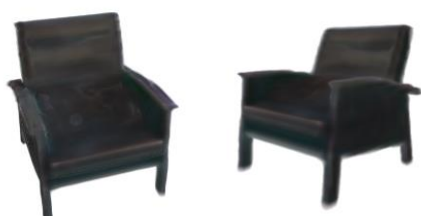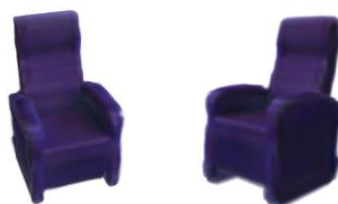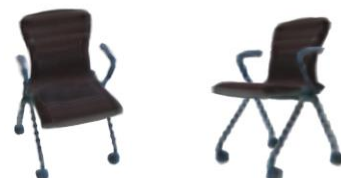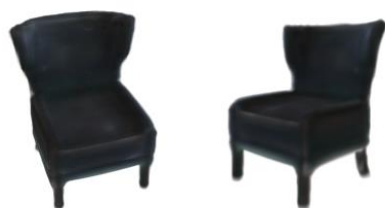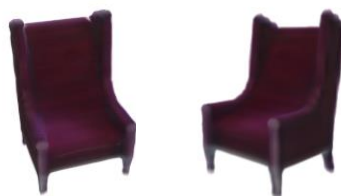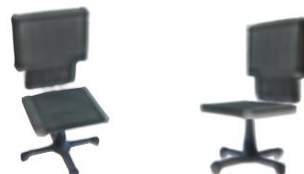

**a leather chair**

**a purple chair**

**chair with wheels**

**Input view**

**Proposal 1**

**Proposal 2**

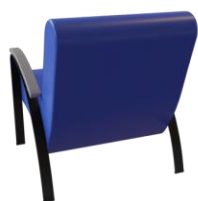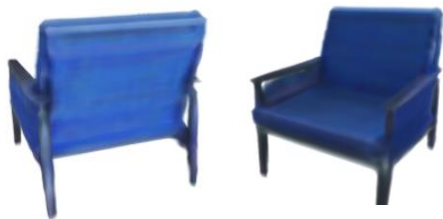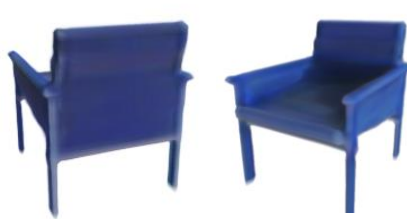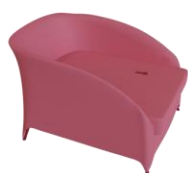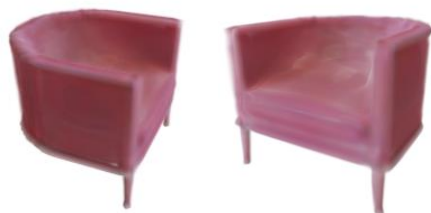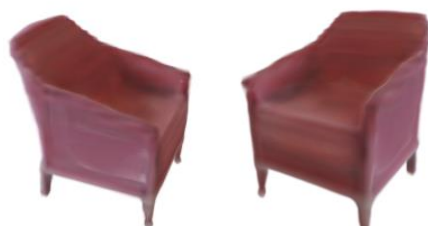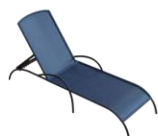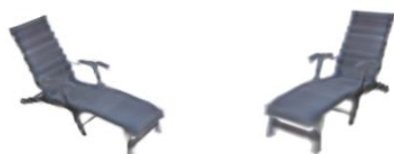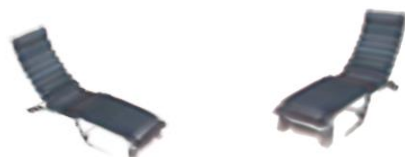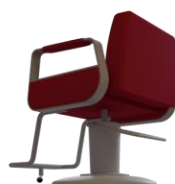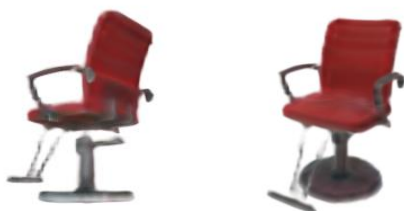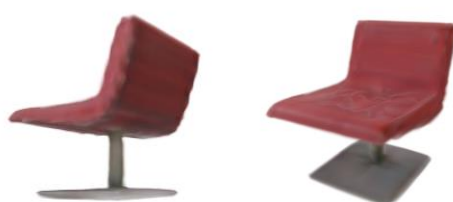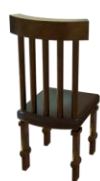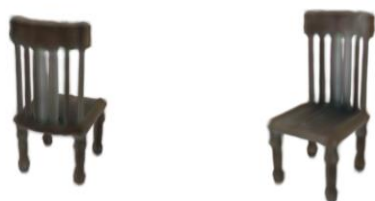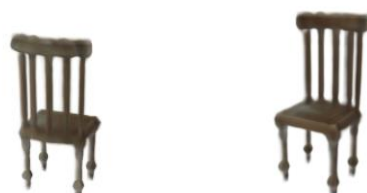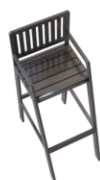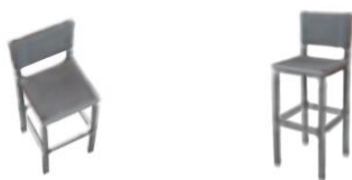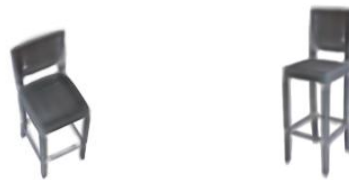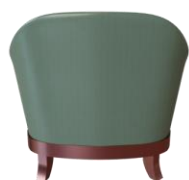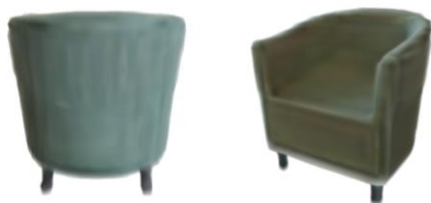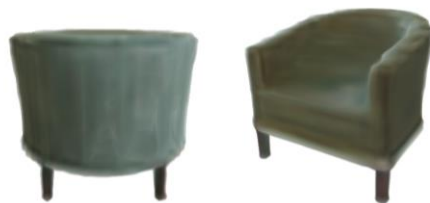

**Input view**

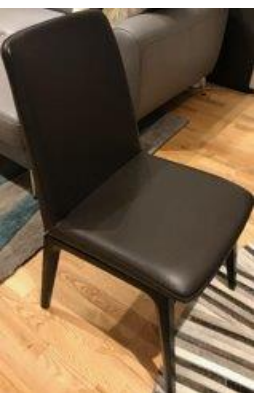

**Proposal 1**

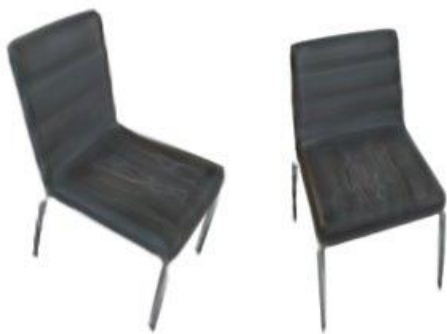

**Proposal 2**

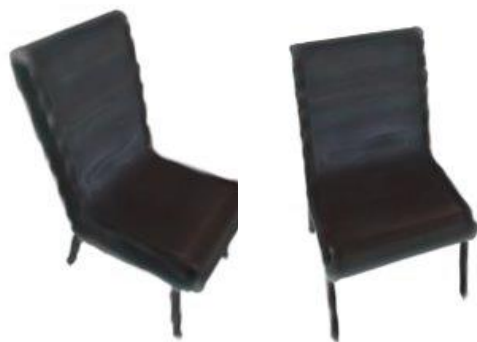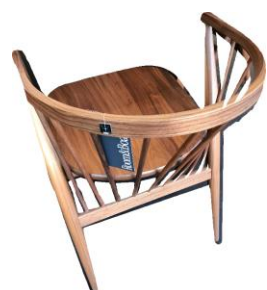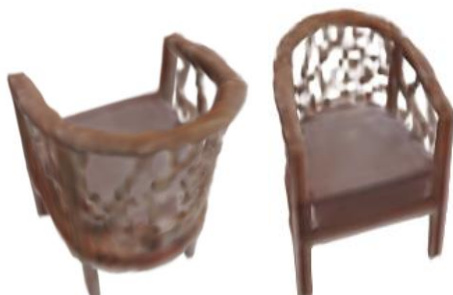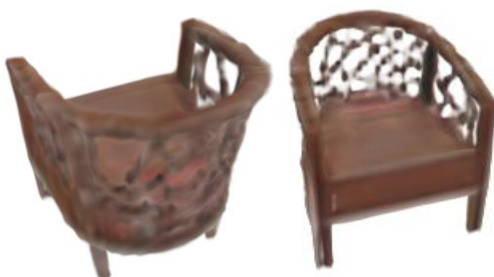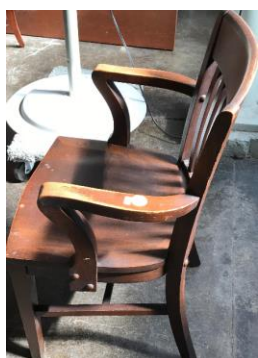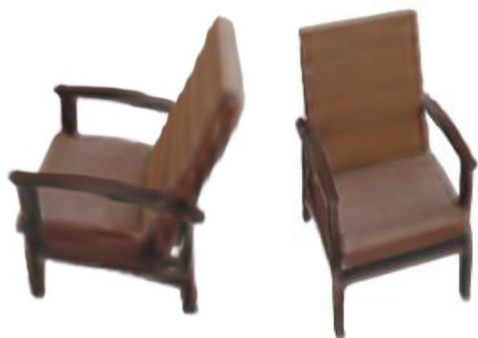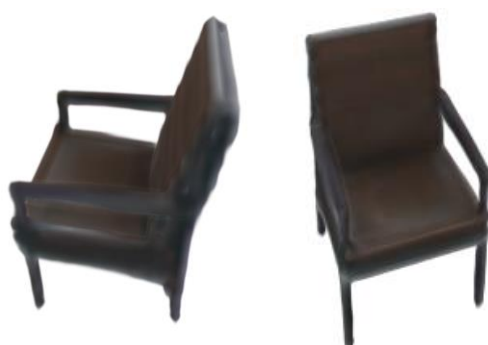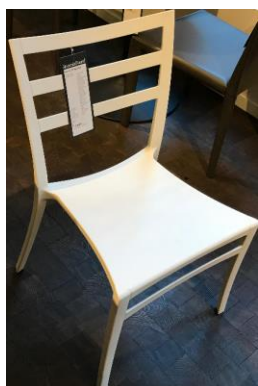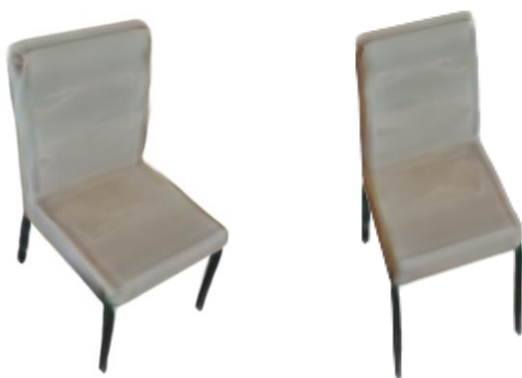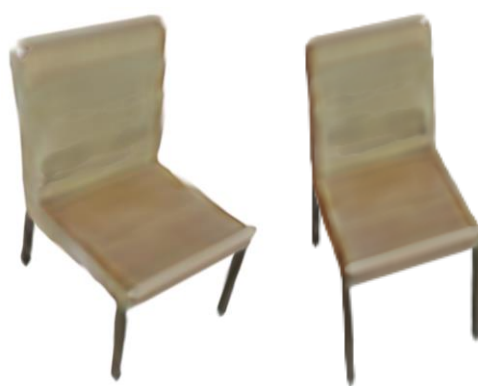

Supplement: Supplementary file 2 [file 2d_comparison.pdf]
