# Supplementary material for: DiffRF: Rendering-Guided 3D Radiance Field Diffusion
Source: arXiv:2212.01206 source file (2023-03-27)

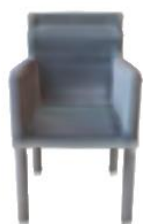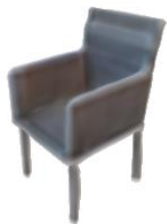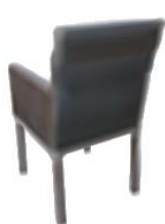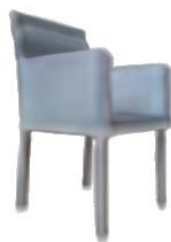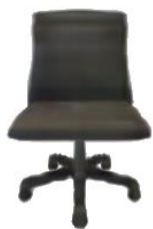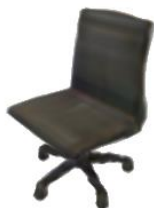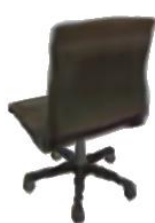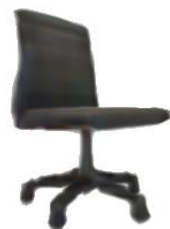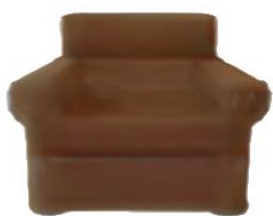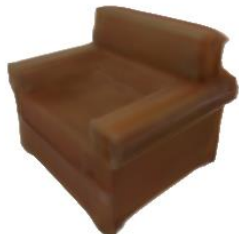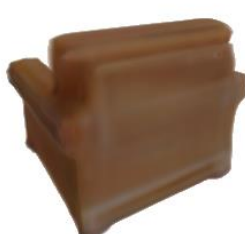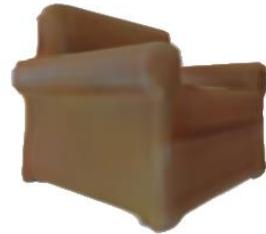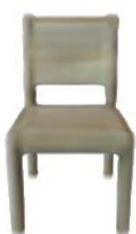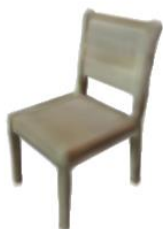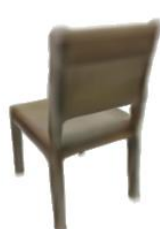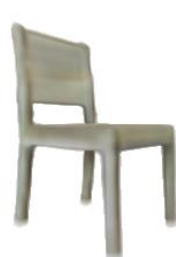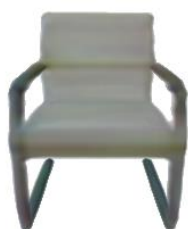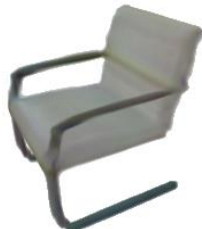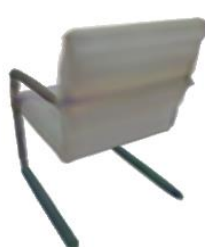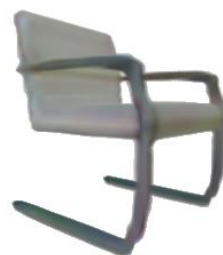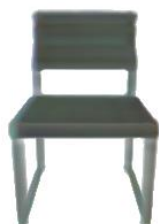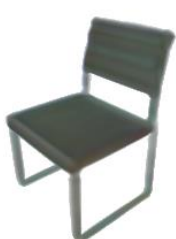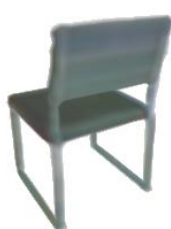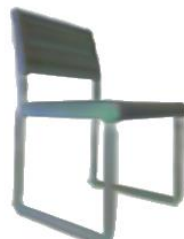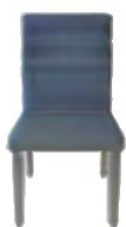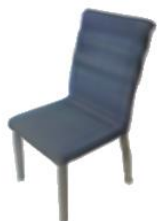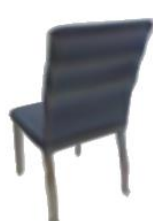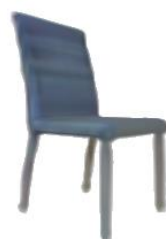

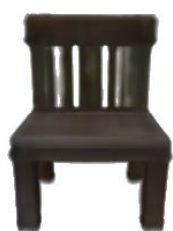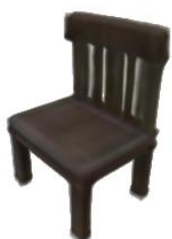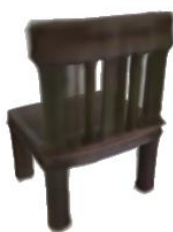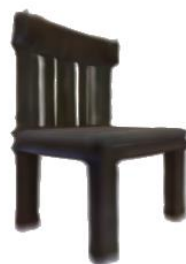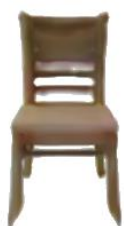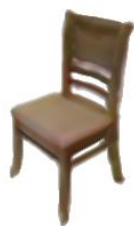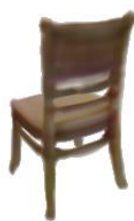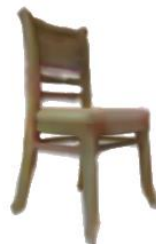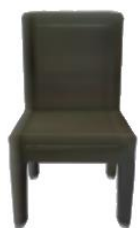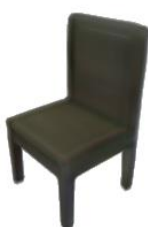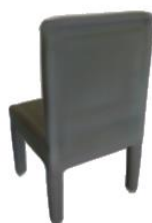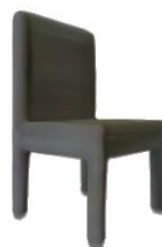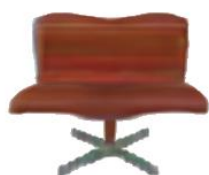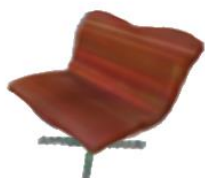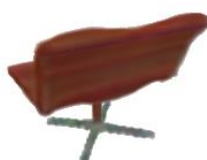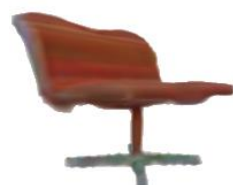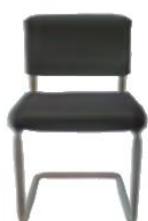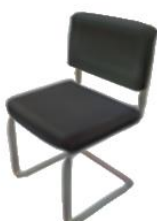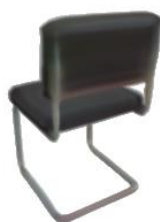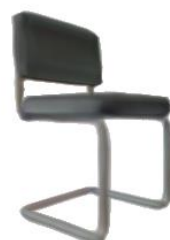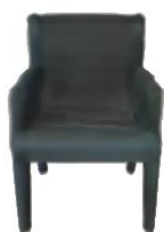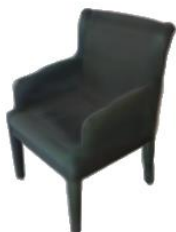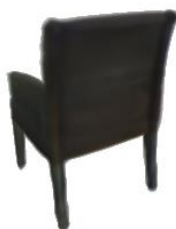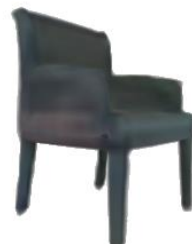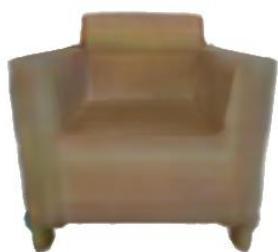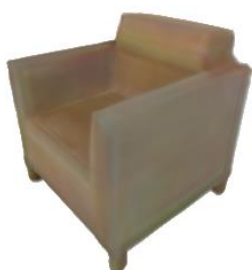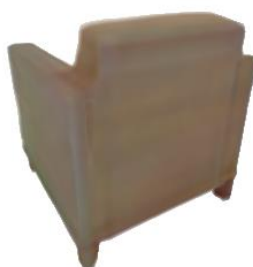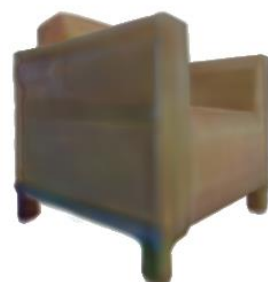

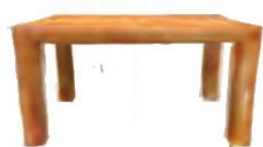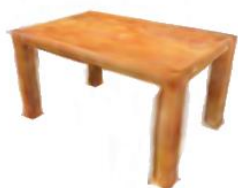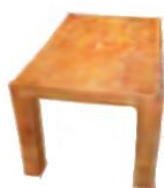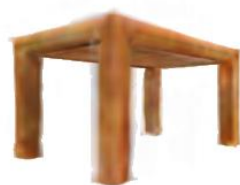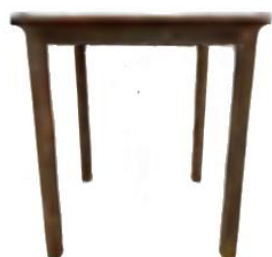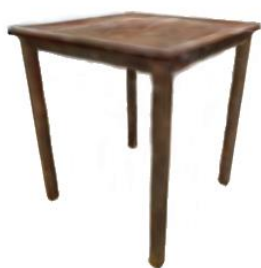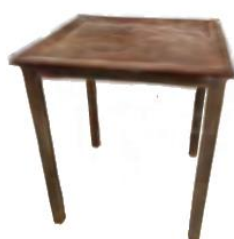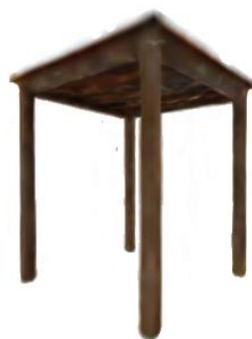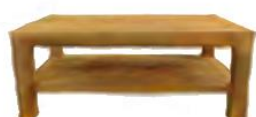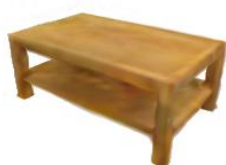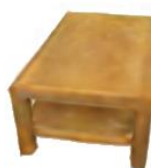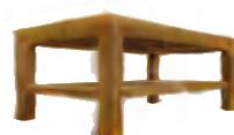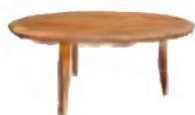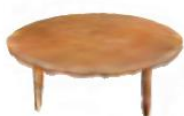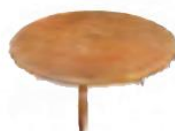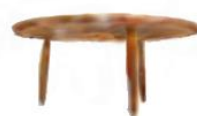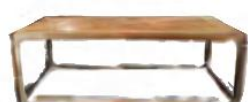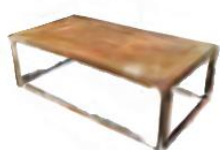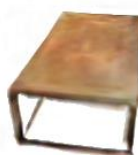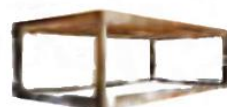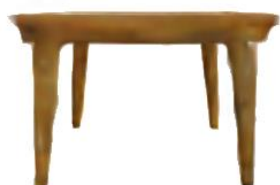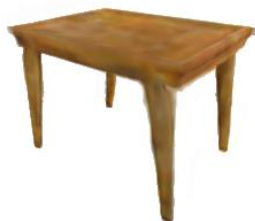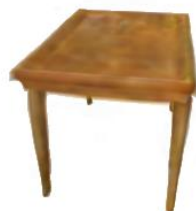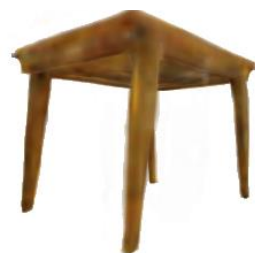

Supplement: Supplementary file 3 [file addition_res0.pdf]
