# Supplementary material for: DiffRF: Rendering-Guided 3D Radiance Field Diffusion
Source: arXiv:2212.01206 source file (2023-03-27)

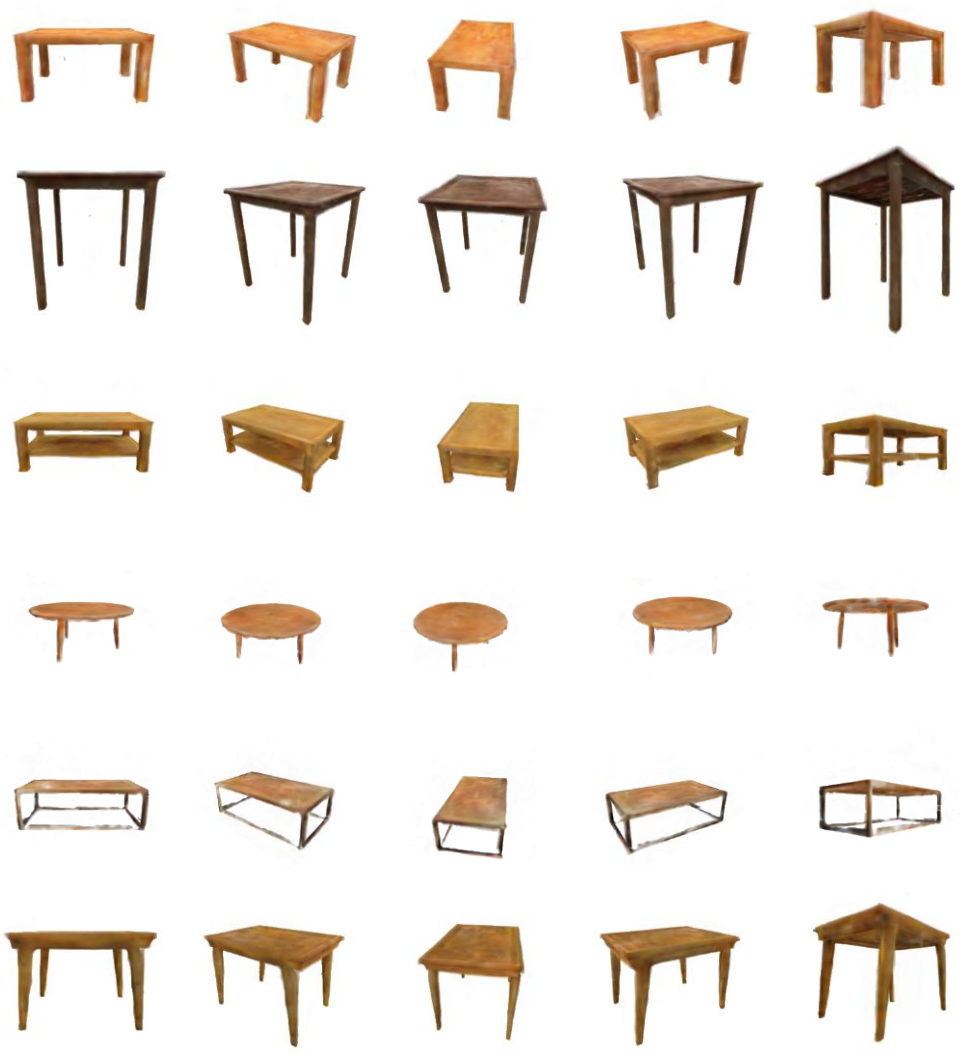

$\pi$ -GAN

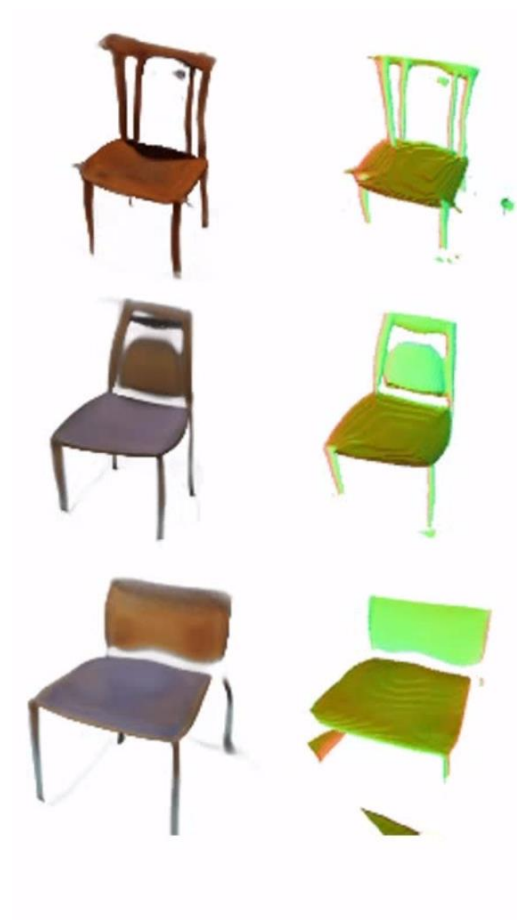

EG3D

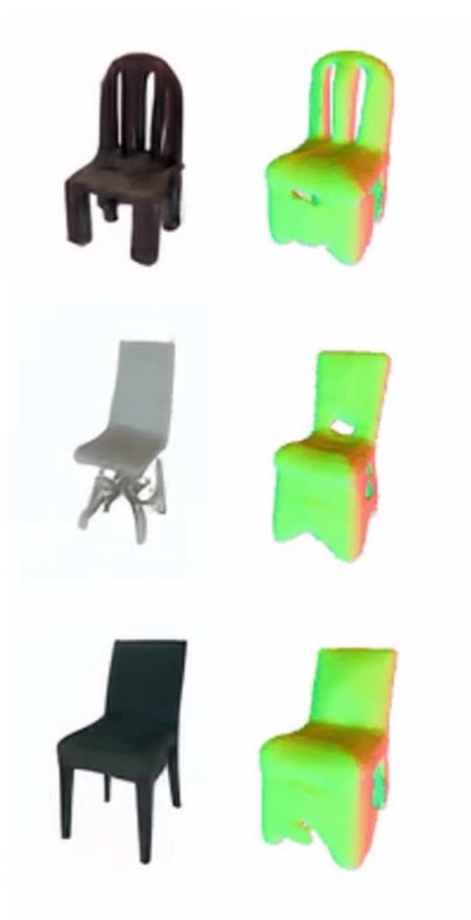

DiffRF

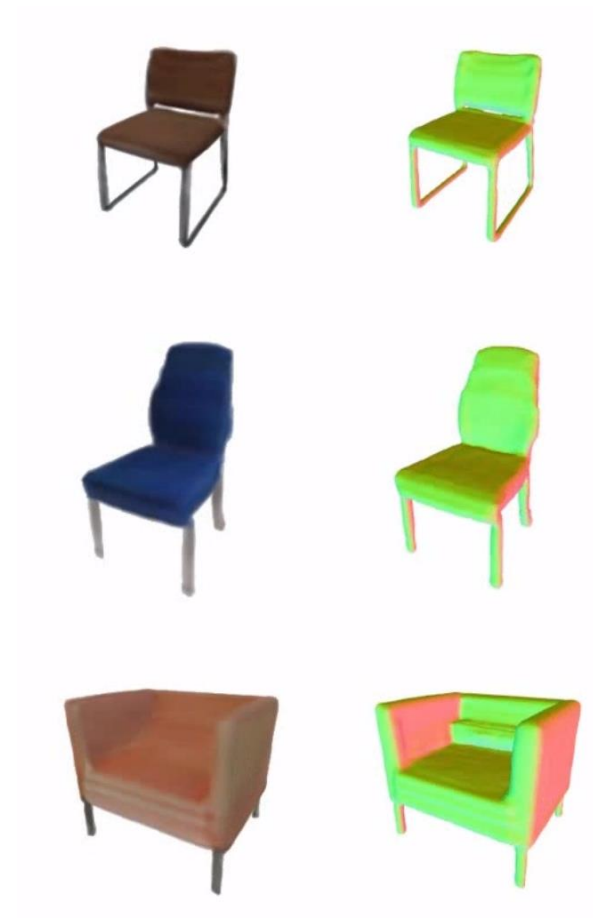

$\pi$ -GAN

EG3D

DiffRF

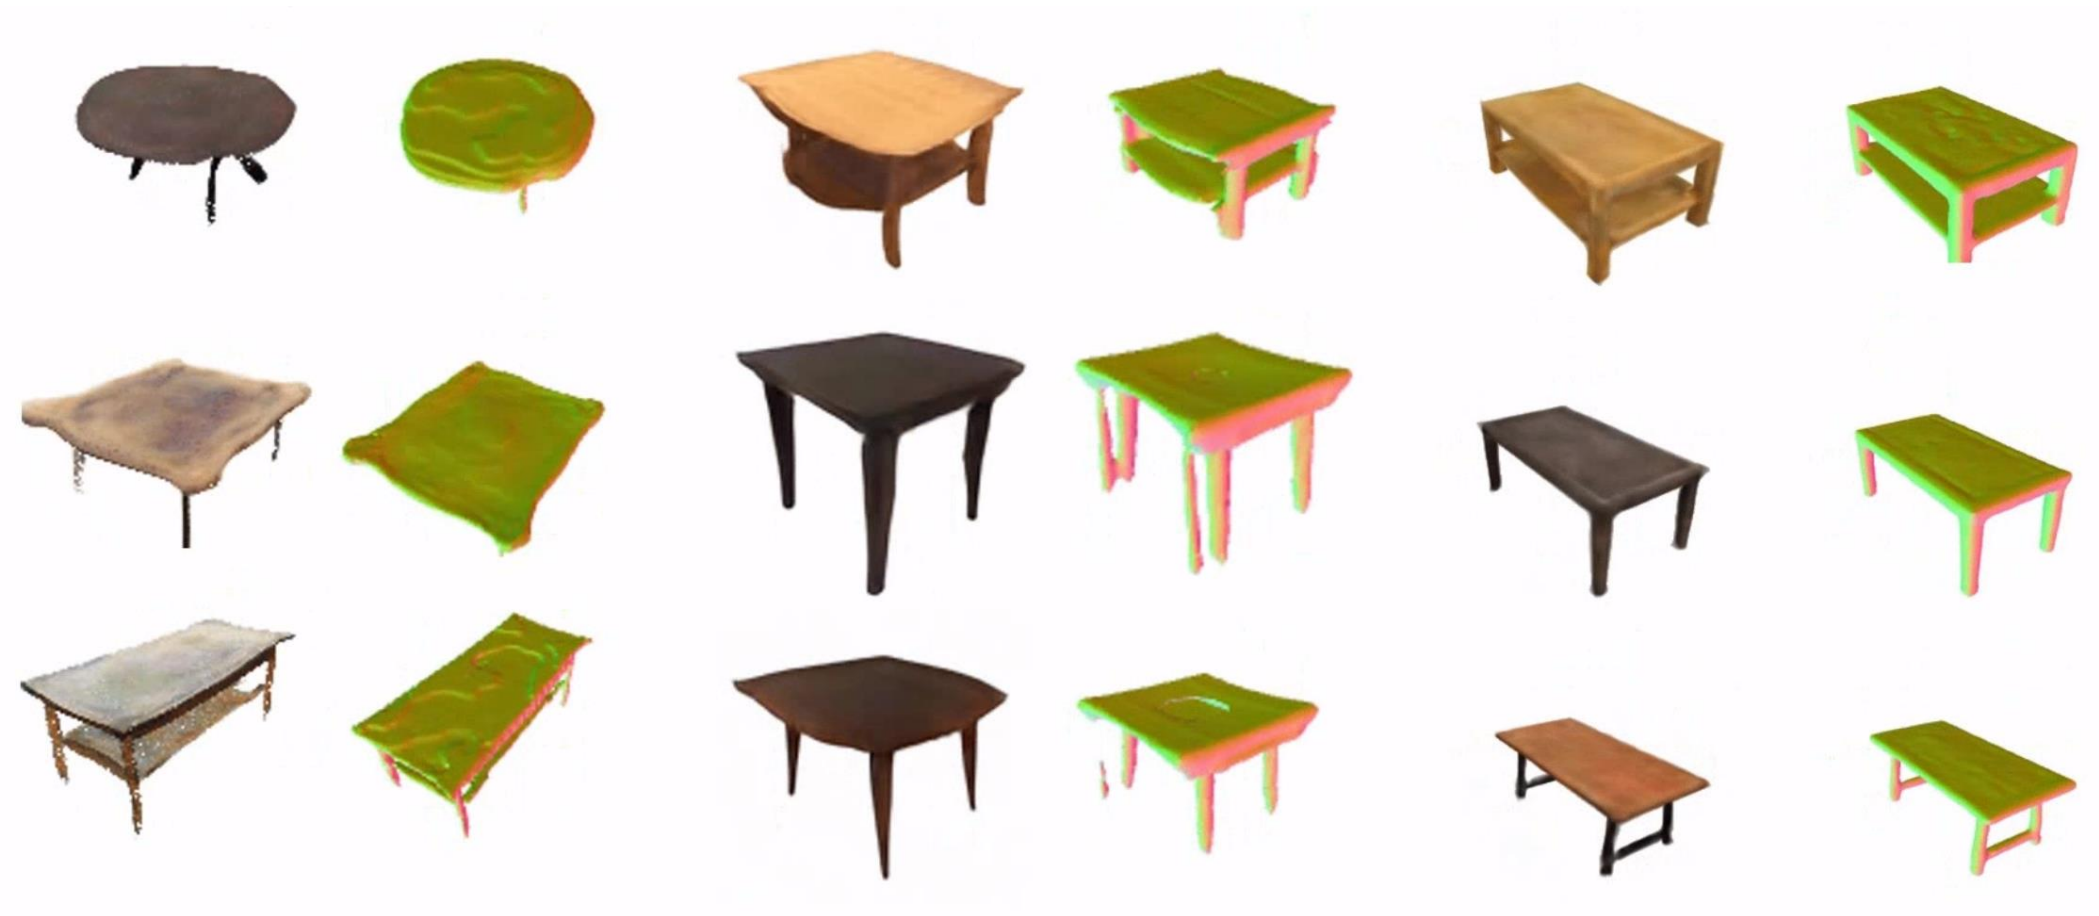

Supplement: Supplementary file 4 [file addition_res1.pdf]
